# Supplementary material for: A Multimodal and Multi-centric Head and Neck Cancer Dataset for Segmentation, Diagnosis and Outcome Prediction
Source: arXiv:2509.00367 source file (2025-09-20)
Supplement: Supplementary file 1 [file supplementary.tex]

\begin{figure}[p]
\centering

% Row 1
\begin{subfigure}[c]{0.3\textwidth}
    \centering
\includegraphics[height=3.5cm,valign=c]{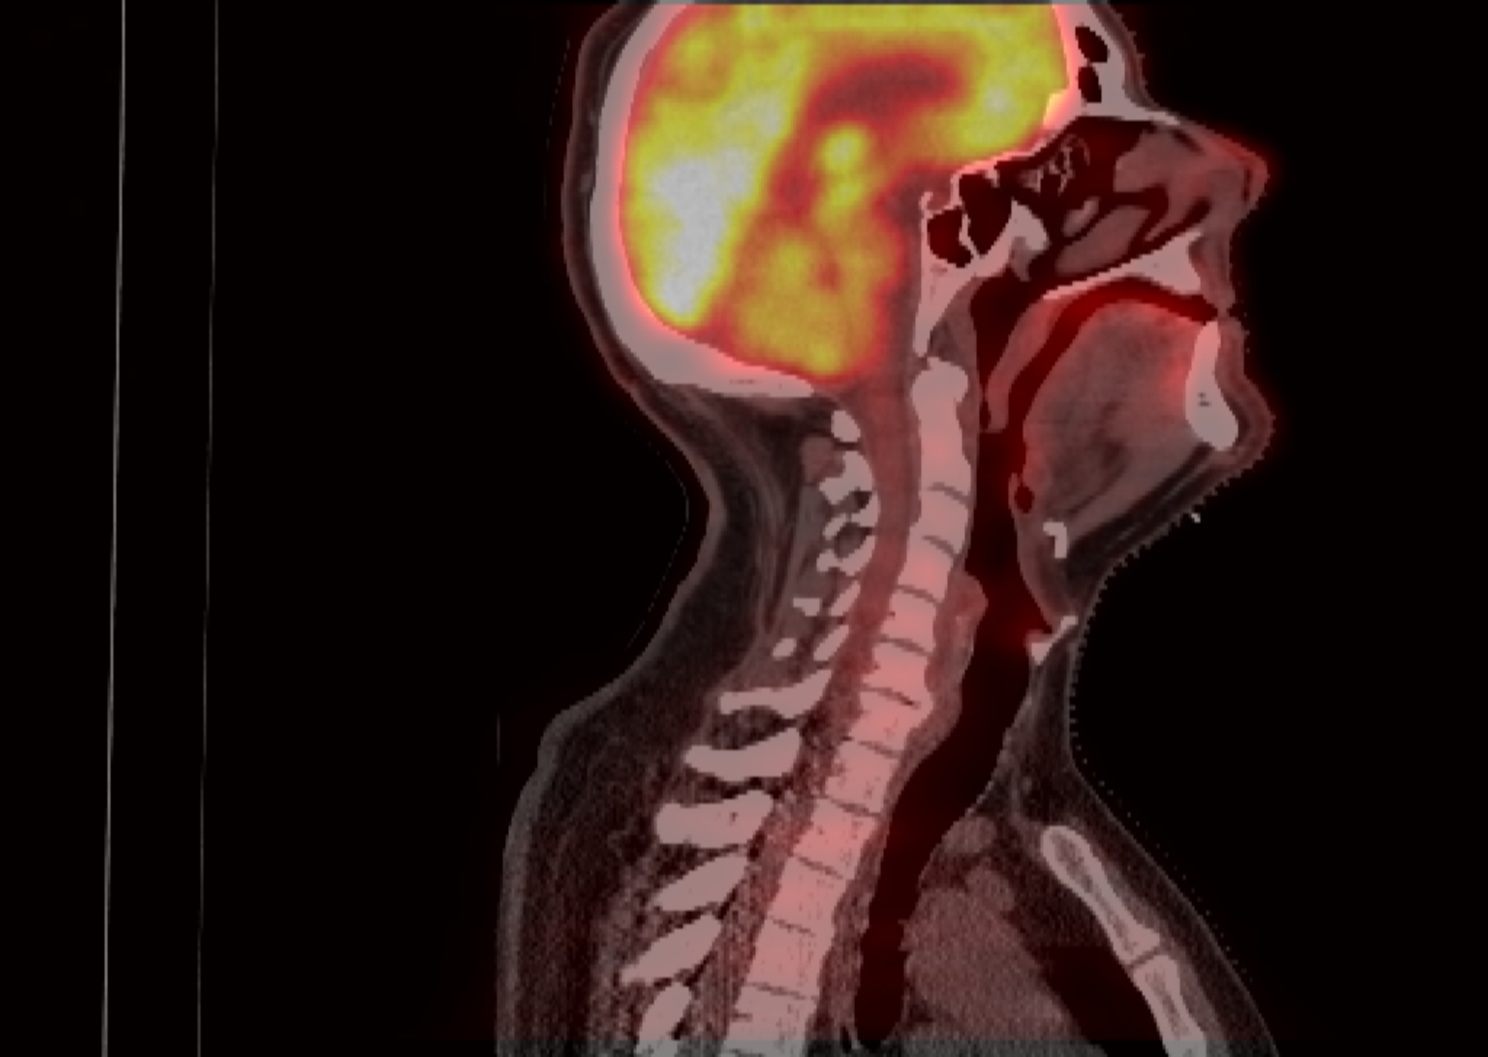}
    \caption{CHUM}
\end{subfigure}
\hfill
\begin{subfigure}[c]{0.3\textwidth}
    \centering
    \includegraphics[height=3.5cm]{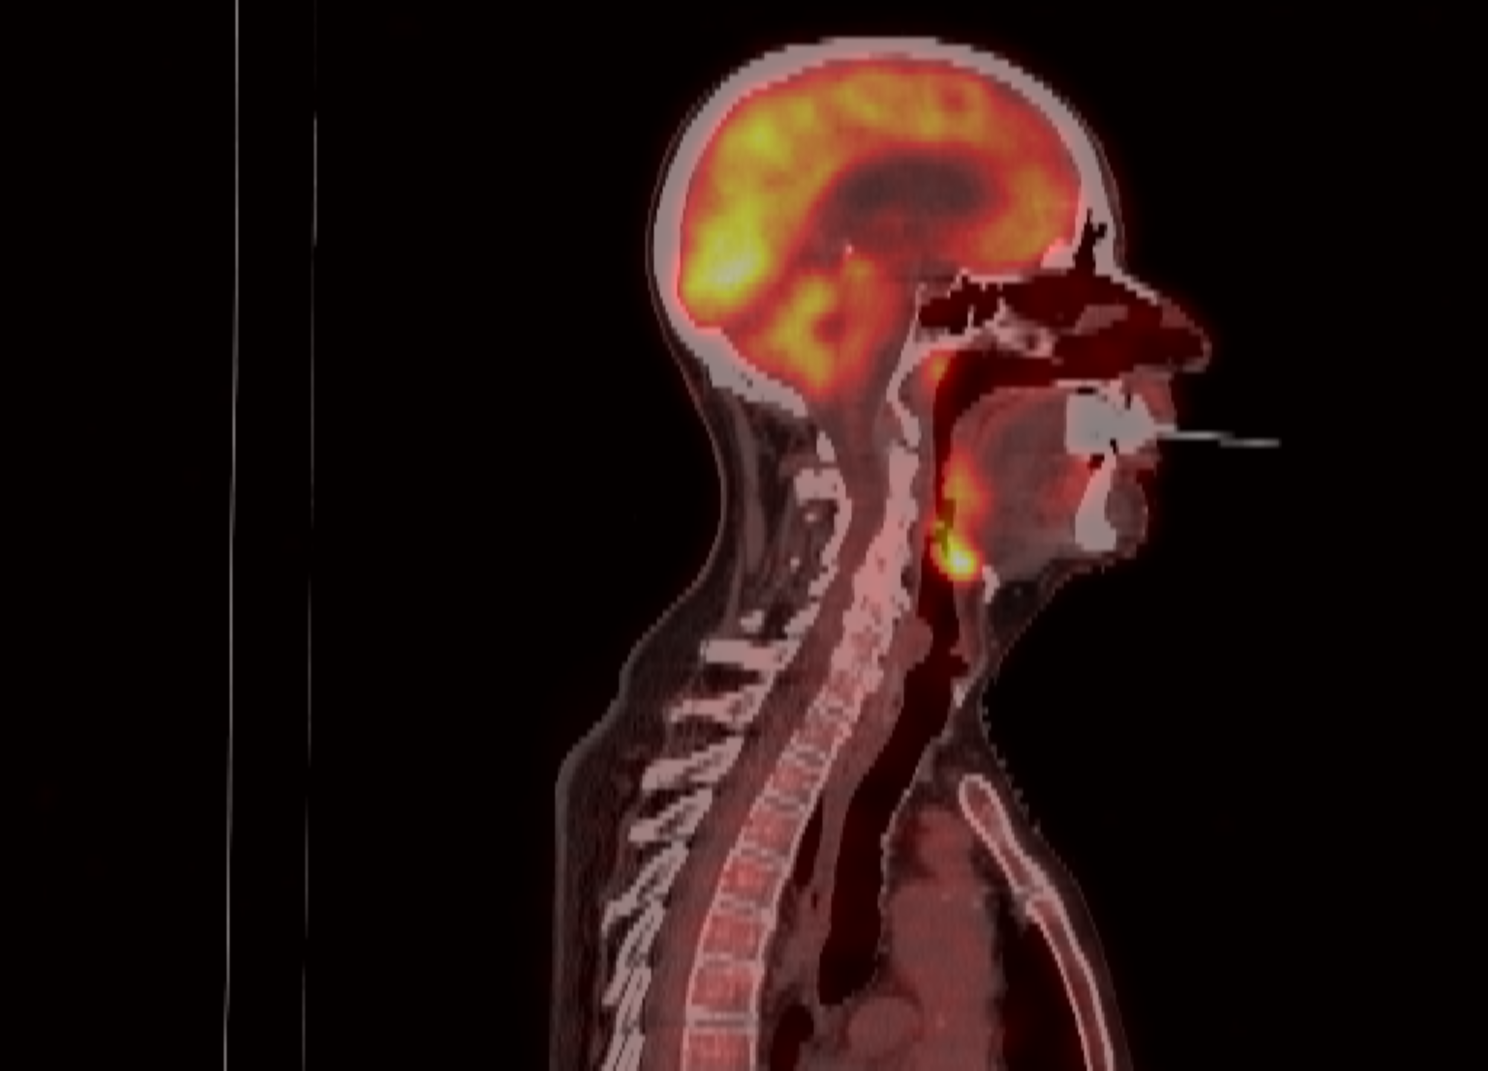}
    \caption{CHUS}
\end{subfigure}
\hfill
\begin{subfigure}[c]{0.3\textwidth}
    \centering
    \includegraphics[height=3.5cm]{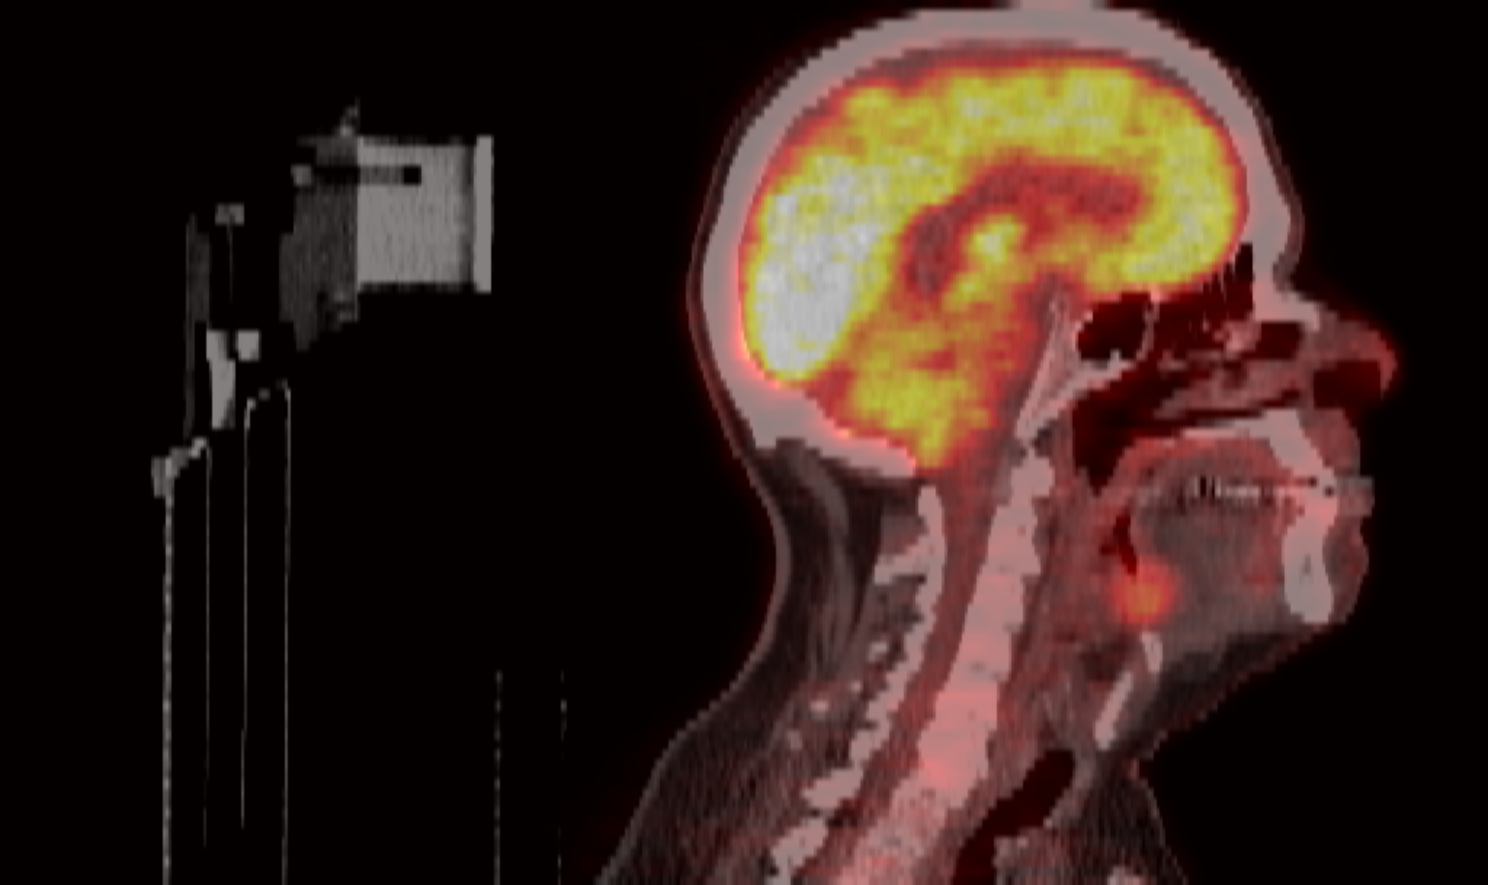}
    \caption{HGJ}
\end{subfigure}

\vspace{0.5cm}

% Row 2
\begin{subfigure}[c]{0.3\textwidth}
    \centering
    \includegraphics[height=6cm]{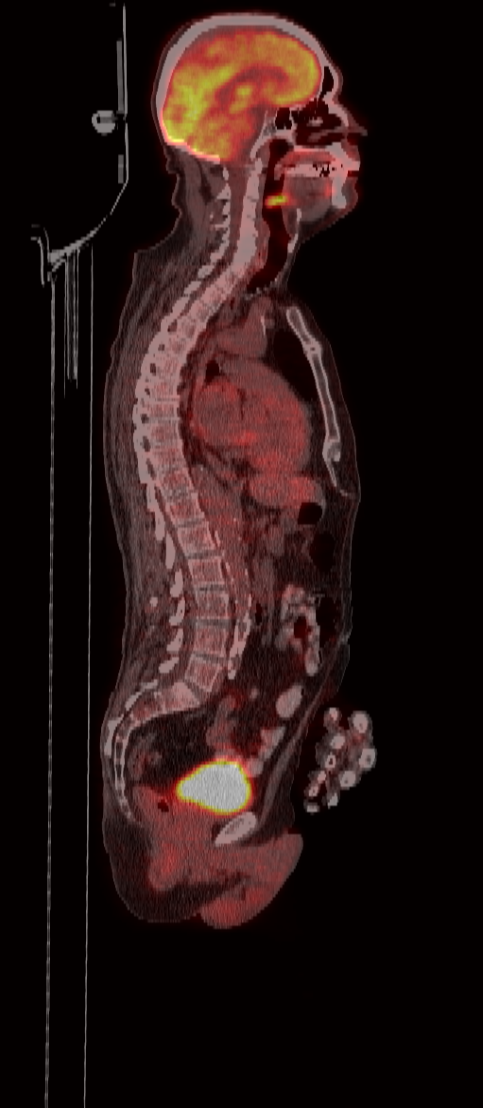}
    \caption{USZ}
\end{subfigure}
\hfill
\begin{subfigure}[c]{0.3\textwidth}
    \centering
    \includegraphics[height=6cm]{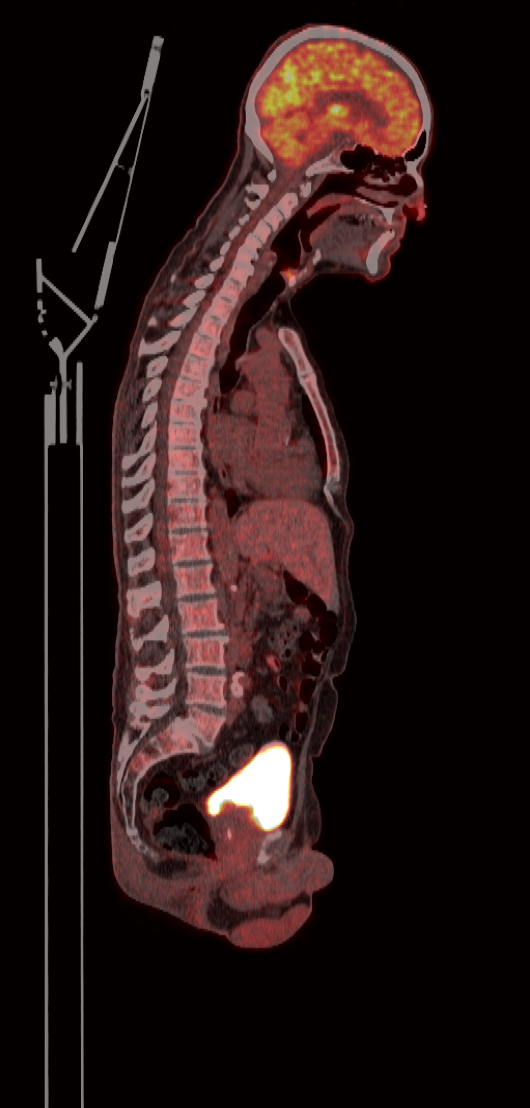}
    \caption{CHUN}
\end{subfigure}
\hfill
\begin{subfigure}[c]{0.3\textwidth}
    \centering
    \includegraphics[height=6cm]{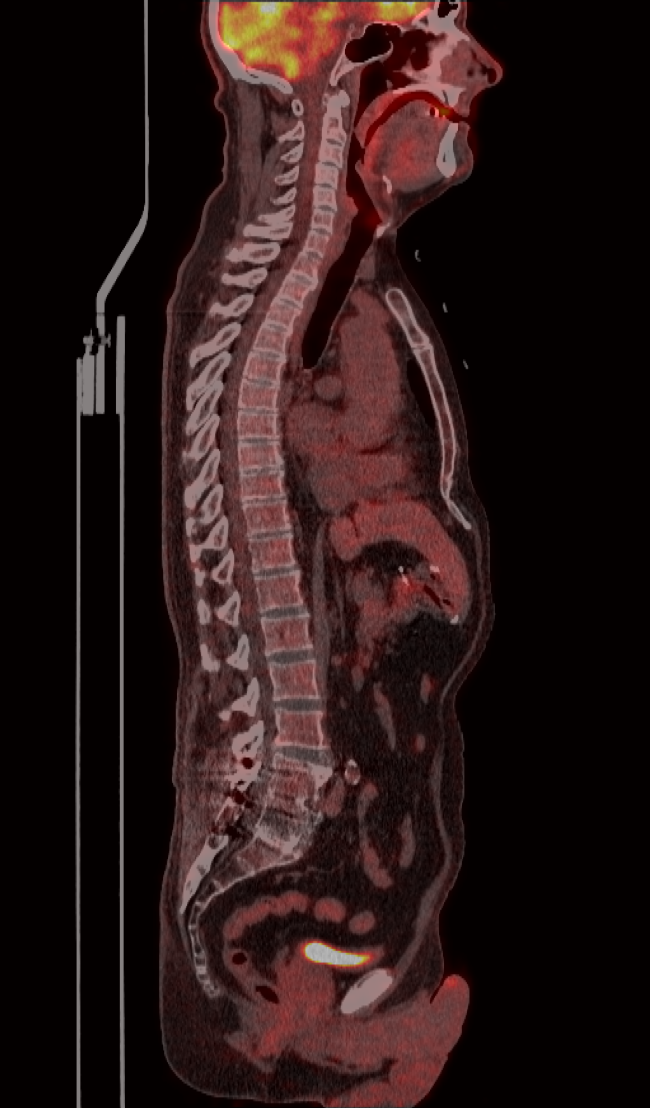}
    \caption{CHUP}
\end{subfigure}

\vspace{0.5cm}

% Row 3
\begin{subfigure}[c]{0.3\textwidth}
    \centering
    \includegraphics[height=3.5cm]{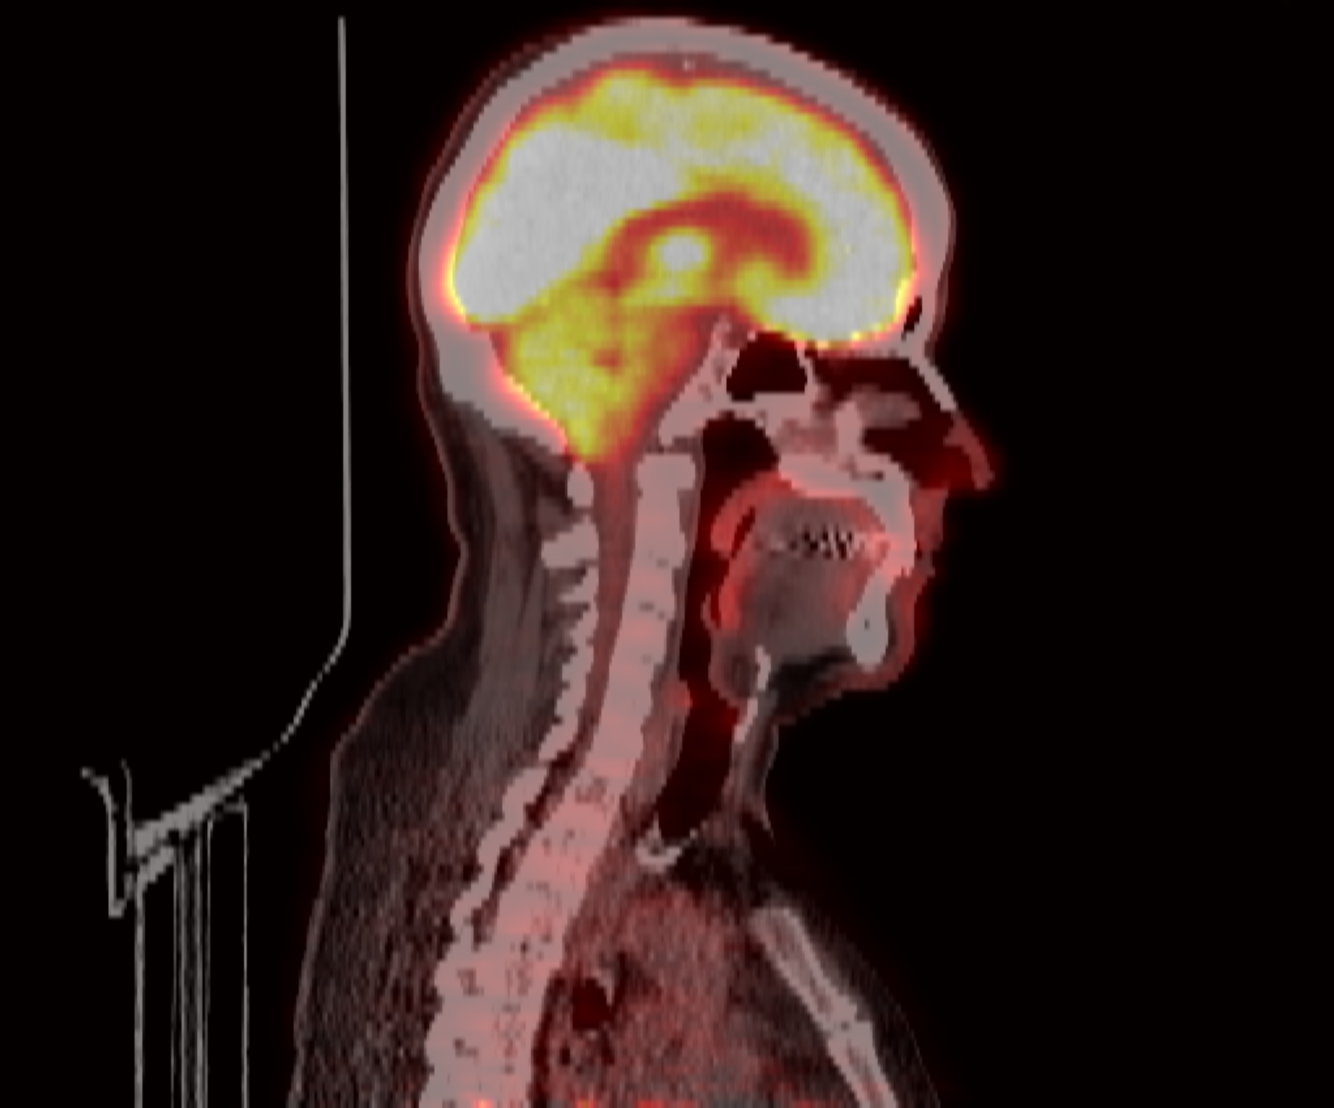}
    \caption{MDA}
\end{subfigure}
\hfill
\begin{subfigure}[c]{0.3\textwidth}
    \centering
    \includegraphics[height=3.5cm]{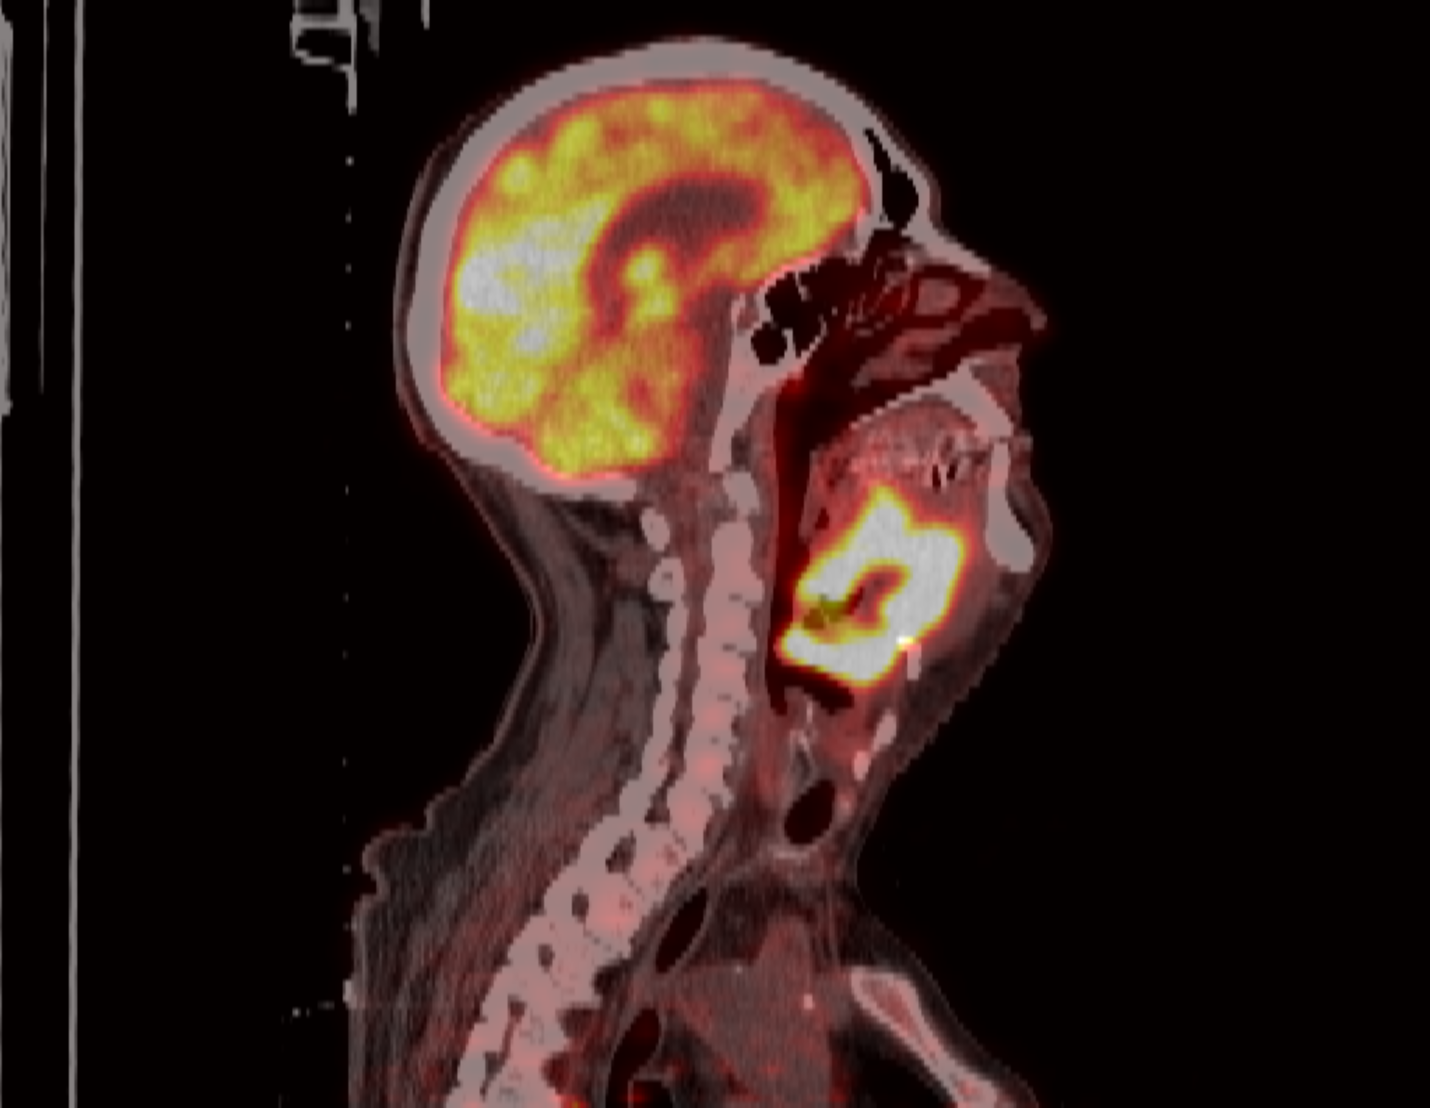}
    \caption{CHB}
\end{subfigure}
\hfill
\begin{subfigure}[c]{0.3\textwidth}
    \centering
    \includegraphics[height=3.5cm]{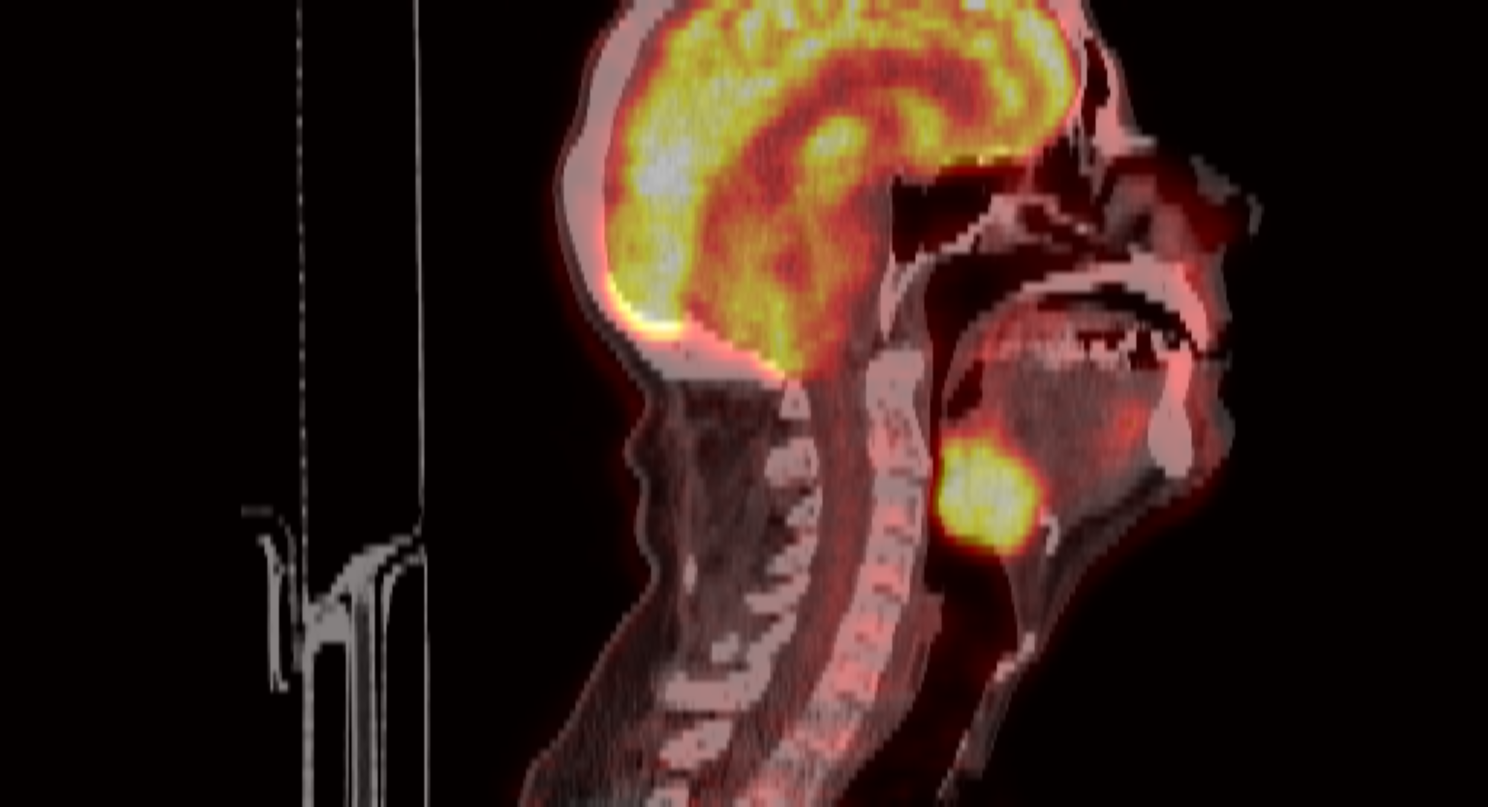}
    \caption{HMR}
\end{subfigure}

\caption{
Sagittal slices of fused PET/CT images from each of the nine centers in the training and validation datasets, showing variability in field-of-view and patient positioning across different centers. The CT images are normalized using a window of $[-140, 260]$ Hounsefield unit and the PET images are normalized using a window of $[0, 12]$ in SUV, rendered using a hot colormap.
}
\label{fig:fused-petct-centers}
\end{figure}
\clearpage

\begin{figure}[!b]
    \centering
    \includegraphics[width=0.6\linewidth]{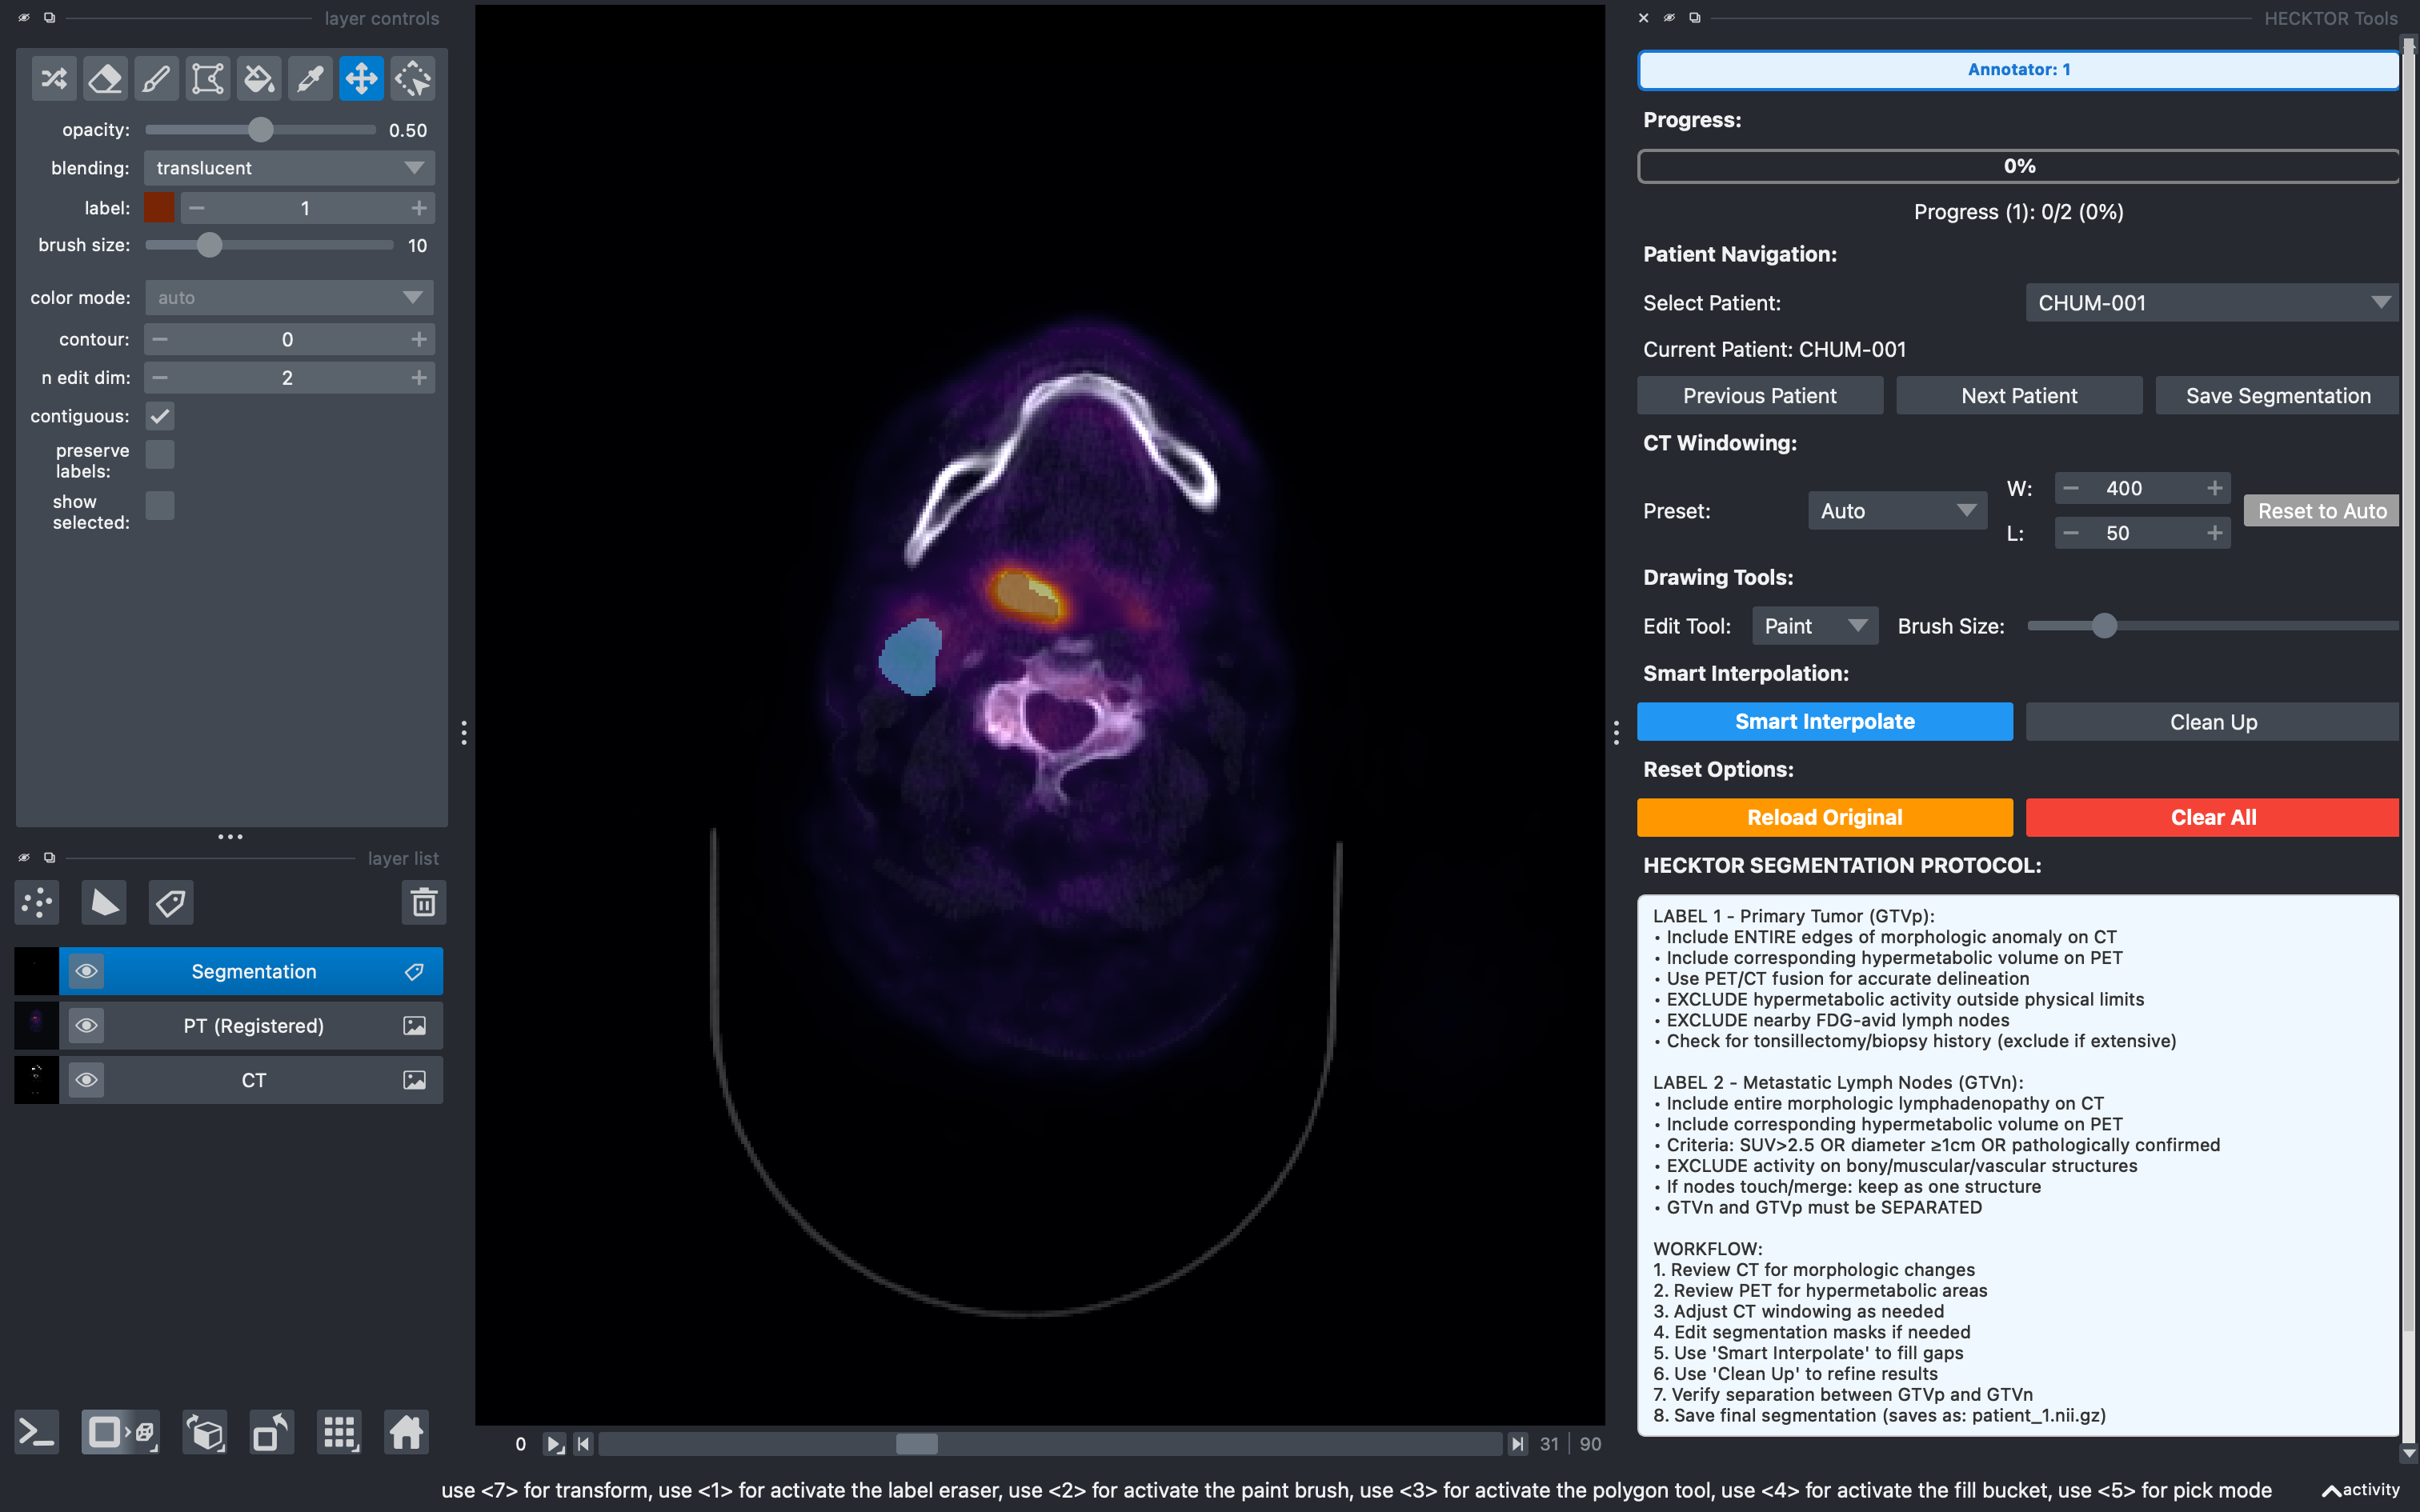}
    \caption{Custom annotation tool developed for the dataset. The interface displays co-registered PET/CT scans with adjustable opacity blending and CT windowing, enabling precise delineation of primary tumors (GTVp) and metastatic lymph nodes (GTVn). Layer controls, patient navigation, segmentation tools, and embedded segmentation protocols are integrated within the platform to guide expert annotators through a standardized workflow, ensuring consistent, high-quality labels across all cases.}
    \label{fig:annotation_tool}
\end{figure}
